# Supplementary material for: Optical Controllable Spin-Polarization in Two Dimensional Altermagnets via Robust Spin-Momentum Locking Excitons
Source: arXiv:2505.23237 ancillary file (2025-11-04)
Supplement: Supplementary file 1 [file SM.pdf]

# Supplemental material for: Optical Controllable Spin-Polarization in 2D Altermagnets via Robust Spin-Momentum Locking Excitons

Jiuyu Sun, Jinzhe Han, Yongping Du,\* and Erjun Kan†  
*MIIT Key Laboratory of Semiconductor Microstructure and Quantum Sensing,  
Nanjing University of Science and Technology, Nanjing 210094, China*  
(Dated: February 20, 2025)

## I. METHODOLOGY DEPENDENT GROUND STATE

To determine the ground state band structures and offer a better starting point for the following BSE calculations, we considered different first-principles methods including PBE+ $U_{\text{eff}}$ , hybrid functionals (HSE06[1] and PBE0[2]). In addition, single-shot GW correction at the level of PBE+ $U_{\text{eff}}$  are also considered, where Hubbard  $U_{\text{eff}}$ 's contribution excluded and included in the self-energies are denoted as GW@ $U_{\text{eff}}$  and GWU@ $U_{\text{eff}}$ , respectively. Note that the QP correction could be extremely dependent on the  $U_{\text{eff}}$ [3], so we considered several values of  $U_{\text{eff}}$ , namely 3.0, 3.5, 4.0 and 4.5 eV. Our (hybrid) density functional theory calculations were performed using the Quantum Espresso package[4] with the optimized norm-conserving Vanderbilt pseudopotentials[5, 6] and a 90 Ry cutoff for the plane wave basis. For the GW step, the cutoff for the dielectric screening is set to be 12 Ry, and the numbers of bands for random-phase approximation (RPA) are set to be 300, 400 and 700 for  $\text{V}_2\text{S}_2\text{O}$  monolayer,  $\text{V}_2\text{Se}_2\text{O}$  monolayer and vdWH, respectively. With the Hybertsen-Louie GPP model[7], the self-energy calculations are performed with 300 and 400 bands for  $\text{V}_2\text{S}_2\text{O}$  monolayer, a convergence test can be found in the next section. All the spin-resolved many-body perturbation calculations[8–10] were performed by using BerkeleyGW package[11, 12]. The ground state and Bethe-Salpeter calculations are performed with  $16 \times 16 \times 1$  and  $32 \times 32 \times 1$   $\mathbf{k}$ -point grids, respectively.

TABLE I. Calculated by different methods, direct band gaps within spin-up at  $\Gamma$  and  $X$  ( $E_g@ \Gamma$ ), spin-splitting energy in valence and conduction bands ( $\Delta_{\text{VB}}^{\uparrow\downarrow}$  and  $\Delta_{\text{CB}}^{\uparrow\downarrow}$ ), as well as GW corrections ( $\Delta E_g$ ) to the band gaps based on different  $U_{\text{eff}}$ .

|                | $E_g@ \Gamma$ | $\Delta E_g@ \Gamma$ | $E_g@ X$ | $\Delta E_g@ X$ | $\Delta_{\text{VB}}^{\uparrow\downarrow}$ | $\Delta_{\text{CB}}^{\uparrow\downarrow}$ |
|----------------|---------------|----------------------|----------|-----------------|-------------------------------------------|-------------------------------------------|
| HSE06          | 3.34          | -                    | 1.05     | -               | 0.53                                      | 1.09                                      |
| PBE0           | 3.30          | -                    | 1.77     | -               | 0.50                                      | 1.10                                      |
| PBE+ $U = 3.0$ | 2.00          | -                    | 0.56     | -               | 0.55                                      | 1.17                                      |
| GW@ $U = 3.0$  | 3.57          | 1.56                 | 1.92     | 1.37            | -0.78                                     | 1.14                                      |
| GWU@ $U = 3.0$ | 5.11          | 3.10                 | 3.19     | 2.62            | -0.37                                     | 1.19                                      |
| PBE+ $U = 3.5$ | 2.00          | -                    | 0.81     | -               | -0.70                                     | 1.20                                      |
| GW@ $U = 3.5$  | 3.82          | 1.82                 | 2.18     | 1.36            | -0.82                                     | 1.15                                      |
| GWU@ $U = 3.5$ | 5.33          | 3.33                 | 3.59     | 2.78            | -0.25                                     | 1.23                                      |
| PBE+ $U = 4.0$ | 2.01          | -                    | 1.02     | -               | 0.83                                      | 1.23                                      |
| GW@ $U = 4.0$  | 4.05          | 2.04                 | 2.34     | 1.32            | -0.80                                     | 1.17                                      |
| GWU@ $U = 4.0$ | 5.51          | 3.50                 | 3.91     | 2.89            | -0.15                                     | 1.27                                      |
| PBE+ $U = 4.5$ | 2.17          | -                    | 1.28     | -               | 0.76                                      | 1.27                                      |
| GW@ $U = 4.5$  | 4.35          | 2.18                 | 2.48     | 1.20            | -0.77                                     | 1.24                                      |
| GWU@ $U = 4.5$ | 5.70          | 3.53                 | 4.26     | 2.98            | 0.02                                      | 1.34                                      |

In Table I, we list the calculated results for  $\text{V}_2\text{S}_2\text{O}$  monolayer. Clearly, we found the band gap at either  $\Gamma$  or  $X$  shows a strong dependence on the computational method. Basically, the band gaps increase with  $U_{\text{eff}}$ , for all PBE+ $U_{\text{eff}}$ , GW@ $U_{\text{eff}}$  and GWU@ $U_{\text{eff}}$ , with the GWU@ $U_{\text{eff}}$  yields a larger correction to the PBE+ $U_{\text{eff}}$ . As for an

\* dypnjust@njust.edu.cn.

† ekan@njust.edu.cn

alters magnet, we care more about the spin-splittings ( $\Delta_{\text{VB}}^{\uparrow\downarrow}$  and  $\Delta_{\text{CB}}^{\uparrow\downarrow}$ ) in this work. Notably, we found the  $\Delta_{\text{VB}}^{\uparrow\downarrow}$  has changes qualitatively with the methods. While PBE+U and hybrid functionals show positive  $\Delta_{\text{VB}}^{\uparrow\downarrow}$  (VBM@X is spin-up), the GW results are opposite (VBM@X is spin-dw). We note that the single-shot GW caused crossover of spin-splitting could also be found in the 2D ferromagnetic semiconductors[13, 14]. On the contrary, the conduction bands at X(Y) valleys show robust spin splittings  $\Delta_{\text{CB}}^{\uparrow\downarrow}$  over 1.0 eV, regardless of the computational method. This provides a solid foundation for SML excitons persist at room temperature.

## II. CONVERGENCE TESTS FOR GW

In Table II, we show the convergence behavior of the band gaps at  $\Gamma$  and X in  $\text{V}_2\text{S}_2\text{O}$  monolayer, calculated by various recipes of  $\text{GW}@PBE+U$  ( $U_{\text{eff}} = 4.5$  eV). It shows that the QP gaps are converged to a difference less than 10 meV except for  $\text{GN}+U_{\text{eff}}$ , which is good enough for supporting the discussion on the dependence of ground state levels in the above section.

TABLE II. The values of band gaps at  $\Gamma$  ( $E_g@ \Gamma$ ) and at X valley within spin-up channel ( $E_g^{\uparrow}@X$ ), calculated by different recipes of  $\text{GW}@U_{\text{eff}} = 4.5$  eV, with varying the number of bands (nbands). The labels HL(GN) and HL(GN)+ $U_{\text{eff}}$  denote GW approximations using Hybertsen-Louie[7](Godby-Needs[15]) GPP model with  $U_{\text{eff}}$ 's contribution excluded and included in the self-energies, respectively.

| nbands | $E_g@ \Gamma$ |                      |       |                      | $E_g^{\uparrow}@X$ |                      |       |                      |
|--------|---------------|----------------------|-------|----------------------|--------------------|----------------------|-------|----------------------|
|        | HL            | HL+ $U_{\text{eff}}$ | GN    | GN+ $U_{\text{eff}}$ | HL                 | HL+ $U_{\text{eff}}$ | GN    | GN+ $U_{\text{eff}}$ |
| 300    | 4.354         | 5.703                | 4.724 | 5.900                | 2.479              | 4.262                | 3.156 | 4.679                |
| 350    | 4.341         | 5.690                | 4.714 | 5.880                | 2.482              | 4.263                | 3.163 | 4.770                |
| 400    | 4.344         | 5.693                | 4.717 | 5.884                | 2.486              | 4.263                | 3.165 | 4.791                |

## III. CHOICE OF SCISSORS OPERATOR

In principle, a standard procedure of *ab initio* many-body Green's function calculations for the excitons is a GW QP correction followed by the BSE. However, based on the data above, one can learn that the single-shot GW approximations have a instable performance for  $\text{V}_2\text{X}_2\text{O}$ . In addition, we found that theorists adopted a  $U_{\text{eff}} = 4.6$  eV for  $\text{V}_2\text{Se}_2\text{O}$  monolayer in the original work to fit the bands by HSE06[16], while their co-workers used a much reduced  $U_{\text{eff}} = 1.0$  eV for doped  $\text{V}_2\text{Se}_2\text{O}$  in a recent work to match the bands measured by the experiment. So far, we can not tell which methodology should be used for such correlated systems, potentially Mott-insulators[17].

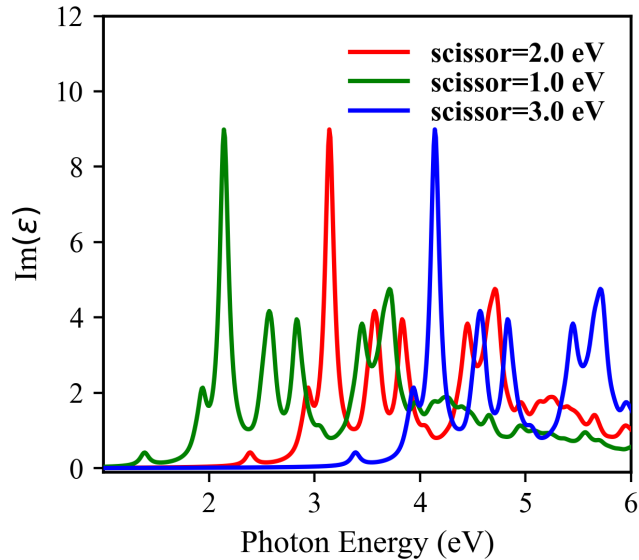

FIG. 1. Optical spectra of  $\text{V}_2\text{S}_2\text{O}$  by BSE with scissor operators of 1.0, 2.0 and 3.0 eV.

Considering the wide utility of Hubbard  $U$  for the strong-correlated materials, we here just use the ground state wavefunction by PBE+ $U$  as the starting point for our BSE calculation. This strategy has been adopted by another theoretical work on the excitons in 2D antiferromagnetic semiconductors[18]. In order to mimic the self-energy effect on the band gap, we further applied a rigid scissor operator to the PBE+ $U$  bands, to grab the physical picture of excitons in a 2D altermagnetic systems with finite-gap. As mentioned above, we find the the QP correction at  $X(Y)$  valleys are sensitive to the methodology, while that at  $\Gamma$  is predictably increasing with the  $U_{\text{eff}}$ . Therefore, after summarizing all the data of QP correction at  $\Gamma$  in the two sections above, we decide to adopt a scissors operator of 2 eV in the BSE calculation for the optical properties. We also tested other values (1 and 3 eV) for the scissors operator, with which the optical spectra are plotted in Figure 1. With the implementation in BerkeleyGW, the value of scissors operator hardly changes the shape of optical spectra.

#### IV. MAGNETIC PROPERTIES OF MONOLAYER $V_2X_2O$ , $X = S, Se, Te$

The magnetic property evaluations were carried out within the framework of density functional theory (DFT) as implemented in the OpenMX code[19–22], employing pseudo-atomic localized basis functions. The basis sets were configured as s2p2d1 for oxygen and sulfur atoms, s3p2d1 for vanadium atoms, and s3p2d2 for selenium and tellurium atoms. Exchange-correlation effects were treated with the Perdew-Burke-Ernzerhof (PBE) generalized gradient approximation[23]. To achieve band gap values consistent with HSE06 calculations, we adopted the DFT+ $U$  approach with a Hubbard  $U$  parameter of 7 eV. Electronic structural relaxations were performed with electronic convergence criteria set to  $10^{-7}$  Hartree, utilizing a plane-wave energy cutoff of 600 Ry and a  $27 \times 27 \times 1$  k-point mesh for Brillouin zone sampling.

Interatomic magnetic interactions were determined through the Green’s function-based magnetic force theory (MFT) using the TB2J code[24], with cross-validation performed via the Jx code[25]. Néel temperature estimates for  $V_2X_2O$  ( $X = S, Se, Te$ ) were derived from Monte Carlo simulations of the Ising model, executed with the open-source mcsolver package[26]. The specific heat curves shown in Fig. 2 indicate their ultra-high Néel temperatures, demonstrating exceptional magnetic stability in these compounds.

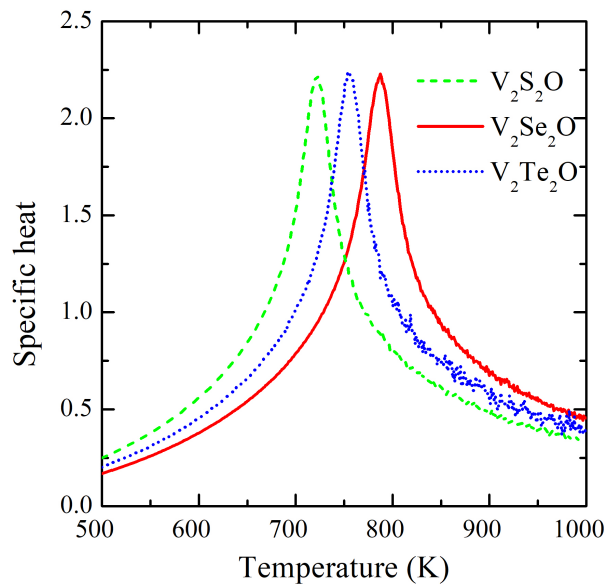

FIG. 2. The specific heat curves of the three materials were calculated using Monte Carlo simulations, revealing ultra-high temperature of magnetic phase transitions: 720 K for  $V_2S_2O$ , 787 K for  $V_2Se_2O$ , and 753 K for  $V_2Te_2O$ .

#### V. RESULTS FOR $V_2SE_2O$ MONOLAYER

In Figure 3, we plotted the calculated results for  $V_2Se_2O$  monolayer with the same information as  $V_2S_2O$  monolayer in the main paper. In general, the two monolayers have similar properties, except some minor disparities. A clear

difference would be the lowest bright exciton, i.e.,  $E_1$ . As shown,  $E_1@V_2Se_2O$  has a higher excitation energy (2.55 eV) than  $E_1@V_2S_2O$ . Instead of transition from the saddle point of top-most valence band along  $\Gamma$ - $X$  in  $V_2S_2O$ , the electron of  $E_1@V_2Se_2O$  hops from the VB valley band on the up-hill way to the summit at  $X$ .

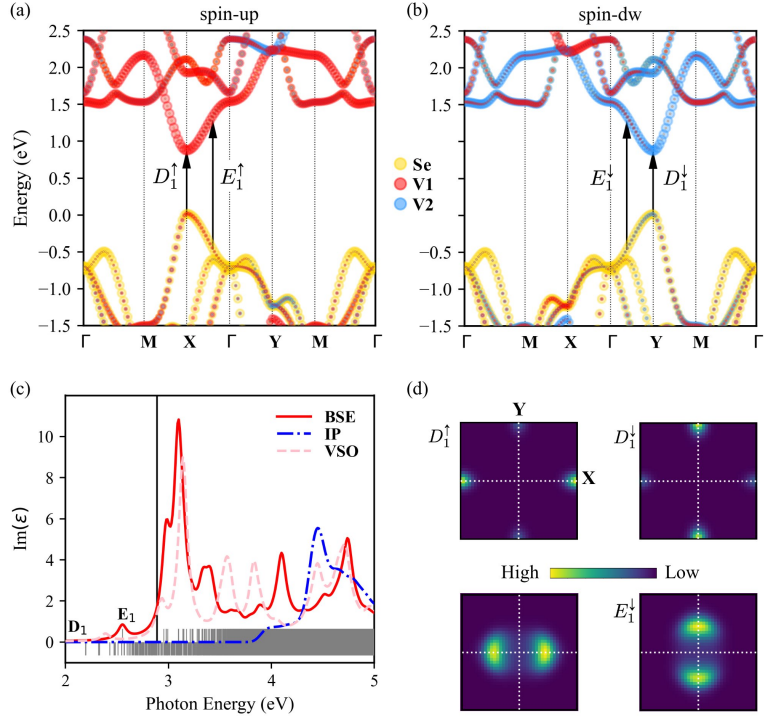

FIG. 3. The calculated results for  $V_2Se_2O$  monolayer. The band structures by PBE+U within (a) spin-up and (b) spin-dw channels, projected onto the V1, V2 and Se atoms with the weights proportional to the radii of the colored circles. Energy zero is at the top of valence band. (c) Optical spectra  $Im(\epsilon)$  by BSE and IP for the light polarization along  $[110]$ . The excitonic energies are reported as vertical grey ticks, and the excitonic energies with module square of dipole moment larger and smaller than  $1 \times 10^{-2}$  are shown separately upon and below zero axis, respectively. The single-particle band gap after the rigid scissor operator are indicated as the black vertical line. The BSE spectrum of  $V_2S_2O$  monolayer is plotted in pink for comparison. (d) Reciprocal-space distributions of optical transitions for selected SML excitons.

## VI. RESULTS FOR OTHER INTERLAYER EXCITONS IN AB-STACKING

- 
- [1] J. Heyd, G. E. Scuseria, and M. Ernzerhof, Erratum: “hybrid functionals based on a screened coulomb potential” [j. chem. phys. 118, 8207 (2003)], The Journal of Chemical Physics **124**, 219906 (2006).
  - [2] C. Adamo and V. Barone, Toward reliable density functional methods without adjustable parameters: The pbe0 model, The Journal of Chemical Physics **110**, 6158 (1999).
  - [3] H. Jiang, R. I. Gomez-Abal, P. Rinke, and M. Scheffler, First-principles modeling of localized  $d$  states with the  $gw@LDA+u$  approach, Physical Review B **82**, 045108 (2010).
  - [4] P. Giannozzi, S. Baroni, N. Bonini, M. Calandra, R. Car, C. Cavazzoni, D. Ceresoli, G. L. Chiarotti, M. Cococcioni, I. Dabo, A. Dal Corso, S. de Gironcoli, S. Fabris, G. Fratesi, R. Gebauer, U. Gerstmann, C. Gougoussis, A. Kokalj, M. Lazzeri, L. Martin-Samos, N. Marzari, F. Mauri, R. Mazzarello, S. Paolini, A. Pasquarello, L. Paulatto, C. Sbraccia, S. Scandolo, G. Sclauzero, A. P. Seitsonen, A. Smogunov, P. Umari, and R. M. Wentzcovitch, Quantum espresso: a modular and open-source software project for quantum simulations of materials, J. Phys. Condens. Matter **21**, 395502 (2009).
  - [5] D. R. Hamann, Optimized norm-conserving vanderbilt pseudopotentials, Phys. Rev. B **88**, 085117 (2013).
  - [6] M. van Setten, M. Giantomassi, E. Bousquet, M. Verstraete, D. Hamann, X. Gonze, and G.-M. Rignanese, The pseudodojo: Training and grading a 85 element optimized norm-conserving pseudopotential table, Computer Physics Communications **226**, 39 (2018).

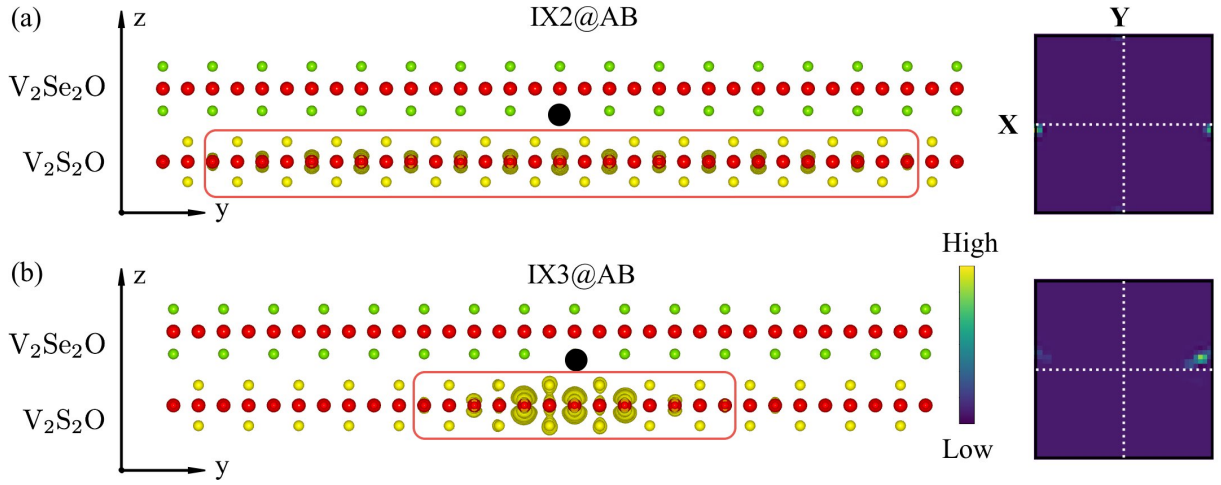

FIG. 4. In spin-up channel, the real-space excitonic wavefunction modulus truncated at 2% of their maximum values, and reciprocal-space distributions of optical transitions for (a)IX<sub>2</sub>@AB and (b)IX<sub>3</sub>@AB. Similar as IX<sub>1</sub>@AB, interlayer distributions are clearly shown for these two excitons. The IX<sub>2</sub>@AB has a larger range of spatial dispersion than IX<sub>2</sub>@AB, and in turn a more confined distribution in the k-space.

- [7] M. S. Hybertsen and S. G. Louie, Electron correlation in semiconductors and insulators: Band gaps and quasiparticle energies, *Phys. Rev. B* **34**, 5390 (1986).
- [8] J.-L. Li, G.-M. Rignanese, E. K. Chang, X. Blase, and S. G. Louie, GW study of the metal-insulator transition of bcc hydrogen, *Phys. Rev. B* **66**, 035102 (2002).
- [9] M. Rohlfing and S. G. Louie, Electron-hole excitations and optical spectra from first principles, *Phys. Rev. B* **62**, 4927 (2000).
- [10] L. X. Benedict and E. L. Shirley, Ab initio calculation of  $\epsilon_2(\omega)$  including the electron-hole interaction: Application to gan and caf<sub>2</sub>, *Phys. Rev. B* **59**, 5441 (1999).
- [11] S. Ismail-Beigi, Truncation of periodic image interactions for confined systems, *Phys. Rev. B* **73**, 233103 (2006).
- [12] J. Deslippe, G. Samsonidze, D. A. Strubbe, M. Jain, M. L. Cohen, and S. G. Louie, Berkeleygw: A massively parallel computer package for the calculation of the quasiparticle and optical properties of materials and nanostructures, *Comput. Phys. Commun.* **183**, 1269 (2012).
- [13] S. Di Sabatino, A. Molina-Sánchez, P. Romaniello, and D. Sangalli, Assignment of excitonic insulators in ab initio theories: The case of NiBr<sub>2</sub>, *Phys. Rev. B* **107**, 115121 (2023), arXiv:2212.11500.
- [14] Z. Jiang, Y. Li, W. Duan, and S. Zhang, Half-Excitonic Insulator: A Single-Spin Bose-Einstein Condensate, *Phys. Rev. Lett.* **122**, 236402 (2019), arXiv:1811.03738.
- [15] R. W. Godby and R. J. Needs, Metal-insulator transition in kohn-sham theory and quasiparticle theory, *Phys. Rev. Lett.* **62**, 1169 (1989).
- [16] H.-Y. Ma, M. Hu, N. Li, J. Liu, W. Yao, J.-F. Jia, and J. Liu, Multifunctional antiferromagnetic materials with giant piezomagnetism and noncollinear spin current, *Nat. Commun.* **12**, 2846 (2021).
- [17] H. Lin, J. Si, X. Zhu, K. Cai, H. Li, L. Kong, X. Yu, and H.-H. Wen, Structure and physical properties of CsV<sub>2</sub>Se<sub>2</sub>xO and V<sub>2</sub>Se<sub>2</sub>O, *Phys. Rev. B* **98**, 075132 (2018).
- [18] M. Birowska, P. E. Faria Junior, J. Fabian, and J. Kunstmann, Large exciton binding energies in MnPS<sub>3</sub> as a case study of a van der Waals layered magnet, *Phys. Rev. B* **103**, L121108 (2021).
- [19] T. e. a. Ozaki, Openmx (open source package for material explorer), <http://www.openmx-square.org>.
- [20] T. Ozaki, Variationally optimized atomic orbitals for large-scale electronic structures, *Phys. Rev. B* **67**, 155108 (2003).
- [21] T. Ozaki and H. Kino, Numerical atomic basis orbitals from h to kr, *Phys. Rev. B* **69**, 195113 (2004).
- [22] T. Ozaki and H. Kino, Efficient projector expansion for the ab initio lcao method, *Phys. Rev. B* **72**, 045121 (2005).
- [23] J. P. Perdew, K. Burke, and M. Ernzerhof, Generalized gradient approximation made simple, *Phys. Rev. Lett.* **77**, 3865 (1996).
- [24] X. He, N. Helbig, M. J. Verstraete, and E. Bousquet, Tb2j: A python package for computing magnetic interaction parameters, *Comput. Phys. Commun.* **264**, 107938 (2021).
- [25] H. Yoon, T. Kim, J.-H. Sim, and M. Han, An open-source software for calculating magnetic interactions based on magnetic force theory, *Comput. Phys. Commun.* **247**, 106927 (2020).
- [26] L. Liu, X. Ren, J. Xie, B. Cheng, W. Liu, T. An, H. Qin, and J. Hu, Magnetic switches via electric field in bn nanoribbons, *Appl. Surf. Sci.* **480**, 300 (2019).
